# Supplementary material for: Collectively Simplifying Trajectories in a Database: A Query Accuracy Driven Approach
Source: arXiv:2311.11204 source file (2023-12-13)
Supplement: Supplementary file 1 [file appendix.tex]

\section*{Additional Experiments} \label{app}

\begin{table*}
\centering
%\vspace*{-2mm}
\caption{Impacts of start level for \texttt{RL4QDTS} (Geolife).}%(end level is set to 12)
\setlength{\tabcolsep}{10pt}
%\vspace*{-3mm}
\begin{tabular}{|c|c|c|c|c|c|c|}
\hline
Start Level &7 &8 &9 &10 &11 \\ \hline
Range Query &$0.557\pm 0.018$ &$0.608\pm 0.019$  &\bm{$0.733\pm 0.018$} &$0.712\pm 0.021$  &$0.686\pm 0.017$  \\ \hline
Time Cost (s) &74.37 &63.28 &61.11 &57.76 &51.83 \\ \hline
\end{tabular}
\label{tab:parameter_gridsize}
%\vspace*{-2mm}
\end{table*}

% \noindent\textbf{Evaluation Platform.}
% We implement \texttt{RL4QDTS} and the baselines in Python 3.6 and Keras 2.2.0. The experiments are conducted on a 10-cores server with an Intel(R) Core(TM) i9-9820X CPU @3.30GHz 64.0GB RAM and an Nvidia GeForce RTX 2080 GPU. 
% The datasets and code is available via the link\footnote{\url{https://www.dropbox.com/sh/ui2yegn2wmok8hs/AAAXRfeKH1R7AHATmMmsW3Cga?dl=0}} enable reproducibility.

\noindent
\textbf{(1) Effectiveness evaluation (varying cube granularity).} We evaluate the effect of the cube size, considering the spatial aspect (i.e., the grid size) in Table~\ref{tab:parameter_gridsize} and the temporal aspect (i.e., time duration) in Table~\ref{tab:parameter_time}, We report the average results of 100 range queries with data distribution on a database with around 1.5 million points. In Table~\ref{tab:parameter_gridsize}, we observe that a moderate size brings the best effectiveness. The reason is that smaller cubes contain fewer candidate points, making the  model miss potential points to be inserted. Further, while larger cubes contain many candidates, the sampled cubes may not capture the query signals accurately, e.g., in the extreme case of setting the grid size to cover the whole database, the capability of cube sampling is removed.
In addition, the time cost increases as the grid size grows since more trajectories need to be maintained within each cube for constructing states. As expected, similar trends can be observed for the temporal duration as shown in Table~\ref{tab:parameter_time}.

\noindent
\textbf{(2) Effectiveness evaluation (varying parameter $K$).} We study the effect of parameter $K$, which controls the state space for decision-making. We construct a database with around 1.5 million points randomly sampled from Geolife, and report the average results of 100 range queries with data distribution and the corresponding running time. In Table~\ref{tab:parameterK}, we observe that the setting of $K=2$ gives the best effectiveness. When $K$ becomes larger, the model performance degrades slightly, since it becomes more difficult to train the model to choose a point among a larger number of candidate points. In addition, the time cost increases as $K$ increases because more time is spent on constructing states. We set $K$ to 2 by default, since this provides a reasonable trade-off between effectiveness and efficiency.

\noindent
\textbf{(3) Training time.} In Table~\ref{tab:training}, we show the training time of \texttt{RL4QDTS} on Geolife with the default settings described in Section~\ref{sec:setup}. We randomly construct 5 training sets with 2,000 to 5,000 trajectories.
For each training set, we report the time cost and effectiveness based on the selected model during the training.
We observe that the training generally takes several hours and that the cost increases almost linearly with the number of trajectories. The effectiveness improves slightly when the number of trajectories exceeds 5,000. We use the setting of 6,000 trajectories to train the \texttt{RL4QDTS} model, which is enough to obtain a good model with a reasonable time cost.

\begin{table*}
\centering
\caption{Impacts of end level for \texttt{RL4QDTS} (Geolife).}%(start level is set to 9)
\setlength{\tabcolsep}{10pt}
%\vspace*{-2mm}
\begin{tabular}{|c|c|c|c|c|c|c|}
\hline
End Level &10 &11 &12 &13 &14 \\ \hline
Range Query &$0.673\pm 0.023$ &$0.681\pm 0.018$  &\bm{$0.733\pm 0.018$} &$0.693\pm 0.019$  &$0.671\pm 0.021$  \\ \hline
Time Cost (s) &50.32 &57.76 &61.11 &62.31 &67.42 \\ \hline
\end{tabular}
\label{tab:parameter_time}
%\vspace*{-2mm}
\end{table*}

\begin{table*}
\centering
\caption{Impacts of parameter $K$ for \texttt{RL4QDTS} (Geolife).}
\setlength{\tabcolsep}{10pt}
%\vspace*{-2mm}
\begin{tabular}{|c|c|c|c|c|c|c|}
\hline
Parameter & $K=1$ & $K=2$ & $K=3$ & $K=4$ & $K=5$ \\ \hline
Range Query &$0.716\pm 0.021$ &\bm{$0.733\pm 0.018$} &$0.724\pm 0.021$ &$0.723\pm 0.023$ &$0.706\pm 0.023$ \\ \hline
Time Cost (s) &59.31 &61.11 &62.43 &63.85 &64.35 \\ \hline
\end{tabular}
\label{tab:parameterK}
%\vspace*{-2mm}
\end{table*}

\begin{table*}
\centering
\caption{Training cost on Geolife.}
%\vspace*{-2mm}
\begin{tabular}{|c|c|c|c|c|c|c|}
\hline
Training size &2,000 &3,000  &4,000  &5,000  &6,000  &7,000 \\ \hline
Range query &$0.687\pm 0.025$ &$0.703\pm 0.017$ &$0.714\pm 0.015$ &$0.724\pm 0.021$ &\bm{$0.733\pm 0.018$} &$0.733\pm 0.018$ \\ \hline
Time Cost (hours)  &0.43 &0.67 &0.88 &1.15 &1.36 &1.55 \\ \hline
\end{tabular}
\label{tab:training}
%\vspace*{-2mm}
\end{table*}
